# Supplementary material for: Towards Real Time Egocentric Segment Captioning for The Blind and Visually Impaired in RGB-D Theatre Images
Source: arXiv:2308.13892 source file (2023-08-26)
Supplement: Supplementary file 1 [file appendix.tex]

\appendix
\section{A Modified VGG-16}
\label{app:vgg}
When training our different models we try including the depth map in images as a fourth channel after mapping depth values into a $[0,255]$ range. 

We modified the features extractor to take input images with 4 channels instead of 3.

This change did not affect the obtained results in any way. 

Conclusion: This additional channel is unnecessary, we decided to abandon this modified model. 

\section{Segment Depth Map Minimum Value}
\label{app:zmin}
Even though we passed depth maps through a mean filter, there were still sparse 0 values which are considered noise, because such values would always be considered as the minimum value of the bounding box of a segment. To solve this issue we had to apply an additional step. 

For each bounding box, we would get the maximum and the mean depth values, then compute an estimation of the radius of the bounding box to get the minimum depth value, as explained in the figure \ref{fig:zmin} and the following equation:
$$
    r = z_{max} - z_{mean}
$$
and so:
$$
    z_{min} = z_{max} - 2 \times r
$$
$$
    z_{min} = z_{max} - 2 \times z_{max} + 2 \times z_{mean}
$$
$$
    z_{min} = 2 \times z_{mean} - z_{max}
$$

\begin{figure}[!ht]
    \centering
    \includegraphics[width=7cm]{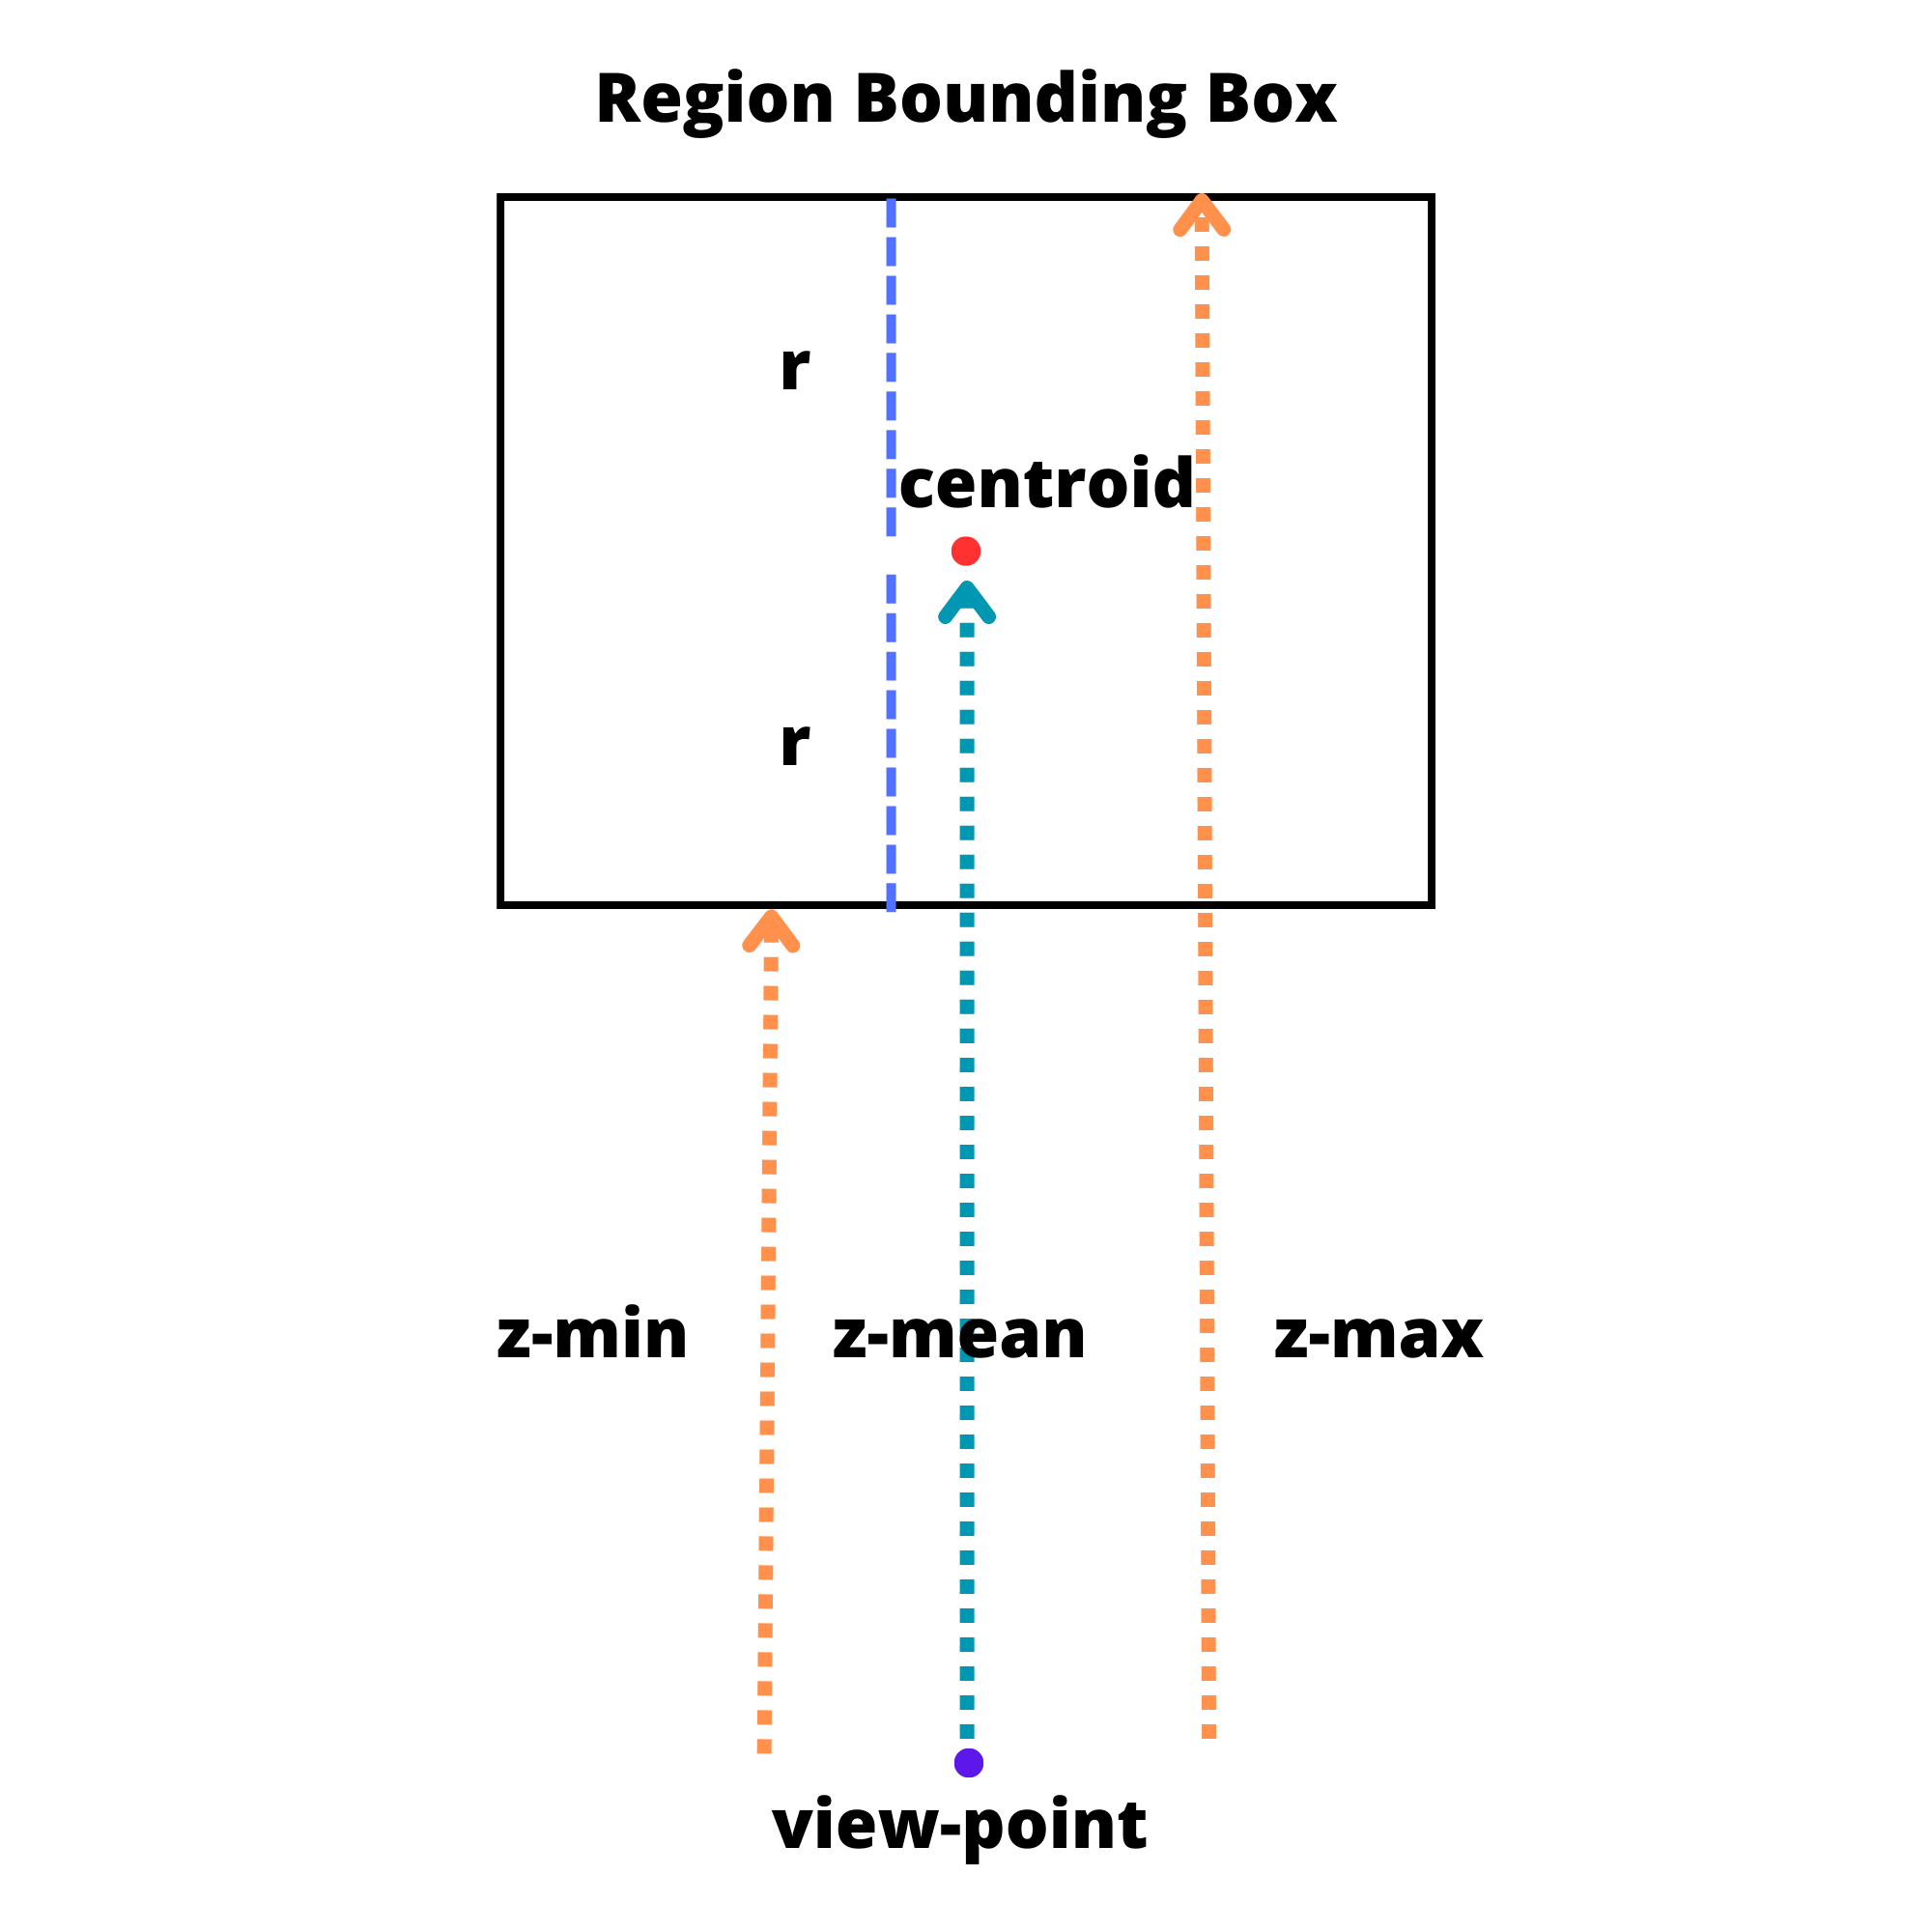}
    \caption{Tackling the zeros minimum values of bounding boxes. An example of a bounding box seen from above.}
    \label{fig:zmin}
\end{figure}
